# Supplementary material for: Enhanced Meta-Learning for Cross-lingual Named Entity Recognition with Minimal Resources
Source: arXiv:1911.06161 source file (2020-07-15)
Supplement: Supplementary file 1 [file supplementary.tex]

\begin{table*}[!hb]
  \centering
    \begin{adjustbox}{max width=\textwidth}
    \begin{tabular}{|c|l|}
      \hline
        \textbf{\#1} & \textbf{Base Model: }... \colorbox[rgb]{0.80, 0.98, 0.85}{[{\scriptsize PER} Fidalgo]} fue elegido para sustituir a \colorbox[rgb]{0.80, 0.98, 0.85}{[{\scriptsize PER} Antonio Gutiérrez]} al frente de la \colorbox[rgb]{0.97, 0.82, 0.80}{Secretaría General}.\\
        % \cline{2-2}
        \multirow{2}{*}{Spanish} & \textbf{Ours: }...  \colorbox[rgb]{0.80, 0.98, 0.85}{[{\scriptsize PER} Fidalgo]} fue elegido para sustituir a \colorbox[rgb]{0.80, 0.98, 0.85}{[{\scriptsize PER} Antonio Gutiérrez]} al frente de la \colorbox[rgb]{0.80, 0.98, 0.85}{[{\scriptsize ORG} Secretaría General]}.\\
        % \cline{2-2}
        & \textbf{Translation in English: }\colorbox[rgb]{1, 1, 1}{... Fidalgo was elected to replace Antonio Gutierrez at the head of the General Secretariat.}\\
        \hline
        \hline
        
        \textbf{\#2} & \textbf{Base Model: }Para la construcción del campo se aprovechará el actual campo de arena ubicado en el patio del \colorbox[rgb]{0.97, 0.82, 0.80}{[{\scriptsize ORG} Colegio Larrea]}.\\
        % \cline{2-2}
        \multirow{2}{*}{Spanish} & \textbf{Ours: }Para la construcción del campo se aprovechará el actual campo de arena ubicado en el patio del \colorbox[rgb]{0.80, 0.98, 0.85}{[{\scriptsize LOC} Colegio Larrea]}.\\
        % \cline{2-2}
        & \textbf{Translation in English: }\colorbox[rgb]{1, 1, 1}{The site will be constructed using the sand dunes currently located on the campus of Larrea College.}\\
        \hline
        \hline
        
        \textbf{\#3} & \textbf{Base Model: }... hebben politie het speelplein \colorbox[rgb]{0.80, 0.98, 0.85}{[{\scriptsize LOC} Redoute]} aan de \colorbox[rgb]{0.97, 0.82, 0.80}{[{\scriptsize PER} Edmond Thieffrylaan]} schoongeveegd van junkies.\\
        % \cline{2-2}
        \multirow{2}{*}{Dutch} & \textbf{Ours: }... hebben politie het speelplein \colorbox[rgb]{0.80, 0.98, 0.85}{[{\scriptsize LOC} Redoute]} aan de \colorbox[rgb]{0.80, 0.98, 0.85}{[{\scriptsize LOC} Edmond Thieffrylaan]} schoongeveegd van junkies.\\
        % \cline{2-2}
        & \textbf{Translation in English: }\colorbox[rgb]{1, 1, 1}{... the police have cleaned up the Redoute playground on Edmond Thieffrylaan from junkies.}\\
        \hline
        \hline
        
        \textbf{\#4} & \textbf{Base Model: }Het eerste bezoek aan de steengroeve \colorbox[rgb]{0.97, 0.82, 0.80}{[{\scriptsize PER} Lemay]} in \colorbox[rgb]{0.80, 0.98, 0.85}{[{\scriptsize LOC} Doornik]} was een overrompelende en chaotische ervaring .\\
        % \cline{2-2}
        \multirow{2}{*}{Dutch} & \textbf{Ours: }Het eerste bezoek aan de steengroeve \colorbox[rgb]{0.80, 0.98, 0.85}{[{\scriptsize LOC} Lemay]} in \colorbox[rgb]{0.80, 0.98, 0.85}{[{\scriptsize LOC} Doornik]} was een overrompelende en chaotische ervaring .\\
        % \cline{2-2}
        & \textbf{Translation in English: }\colorbox[rgb]{1, 1, 1}{The first visit to the Lemay quarry in Doornik was an overwhelming and chaotic experience.}\\
        \hline
        \hline
         
        \textbf{\#5} & \textbf{Base Model: }
        Kurzfristig wurde der Vorgänger \colorbox[rgb]{0.97, 0.82, 0.80}{[{\scriptsize ORG} Krauses]} , \colorbox[rgb]{0.80, 0.98, 0.85}{[{\scriptsize PER} Peter Wünsch]}, zurückgeholt.\\
        % \cline{2-2}
        \multirow{2}{*}{German} & \textbf{Ours: }
        Kurzfristig wurde der Vorgänger \colorbox[rgb]{0.80, 0.98, 0.85}{[{\scriptsize PER} Krauses]} , \colorbox[rgb]{0.80, 0.98, 0.85}{[{\scriptsize PER} Peter Wünsch]}, zurückgeholt.\\
        % \cline{2-2}
        & \textbf{Translation in English: }\colorbox[rgb]{1, 1, 1}{Not long ago, Krauses' predecessor, Peter Wünsch, was taken back.}\\
        \hline
        \hline
        
        \textbf{\#6} & \textbf{Base Model: }
        Im Finale (\colorbox[rgb]{0.97, 0.82, 0.80}{Walpurgisnacht}) übertönte der Chor die Stimmen der Solisten, die Mühe hatten ...\\
        % \cline{2-2}
        \multirow{2}{*}{German} & \textbf{Ours: }
        Im Finale (\colorbox[rgb]{0.80, 0.98, 0.85}{[{\scriptsize MISC} Walpurgisnacht]}) übertönte der Chor die Stimmen der Solisten, die Mühe hatten ...\\
        % \cline{2-2}
        & \textbf{Translation in English: }\colorbox[rgb]{1, 1, 1}{In the final (Walpurgis Night), the choir drowned out the voice of the soloist who had trouble ...}\\
        \hline
        \hline
         
        \textbf{\#7} & \textbf{Base Model: }Nos troupes $<$ nt réalisé de nouveaux progrès sur les hauteurs qui dominent \colorbox[rgb]{0.97, 0.82, 0.80}{[{\scriptsize ORG} Cernav]}.\\
        % \cline{2-2}
        \multirow{2}{*}{French} & \textbf{Ours: }Nos troupes $<$ nt réalisé de nouveaux progrès sur les hauteurs qui dominent \colorbox[rgb]{0.80, 0.98, 0.85}{[{\scriptsize LOC} Cernav]}.\\
        % \cline{2-2}
        & \textbf{Translation in English: }\colorbox[rgb]{1, 1, 1}{Our troops made new progress on the heights that dominate Cernav.}\\
        \hline
        \hline
         
        \textbf{\#8} & \textbf{Base Model: }A 2 heures , route de \colorbox[rgb]{0.97, 0.82, 0.80}{[{\scriptsize PER} Landivisiau]}, course au galop le prix, 30 fr.\\
        % \cline{2-2}
        \multirow{2}{*}{French} & \textbf{Ours: }A 2 heures , route de \colorbox[rgb]{0.80, 0.98, 0.85}{[{\scriptsize LOC} Landivisiau]}, course au galop le prix, 30 fr.\\
        % \cline{2-2}
        & \textbf{Translation in English: }\colorbox[rgb]{1, 1, 1}{At 2 o'clock, road of Landivisiau, galloping race the price, 30 fr.}\\
        \hline
        \hline
        
        \textbf{\#9} & \textbf{Base Model: }
        \begin{CJK}{UTF8}{gbsn}
        在 \colorbox[rgb]{0.80, 0.98, 0.85}{[{\scriptsize LOC} 希腊]} ， 人们 常称 他 为 `` 小 \colorbox[rgb]{0.97, 0.82, 0.80}{奥纳西斯} " 。
        \end{CJK}
        \\
        \multirow{2}{*}{Chinese} & \textbf{Ours: }
        \begin{CJK}{UTF8}{gbsn}
        在 \colorbox[rgb]{0.80, 0.98, 0.85}{[{\scriptsize LOC} 希腊]} ， 人们 常称 他 为 `` 小 \colorbox[rgb]{0.80, 0.98, 0.85}{[{\scriptsize PER} 奥纳西斯]} " 。
        \end{CJK}
        \\
        & \textbf{Translation in English: }\colorbox[rgb]{1, 1, 1}{In Greece, he is often called "Little Onassis".}\\
        \hline
        \hline
        
        \textbf{\#10} & \textbf{Base Model: }
        \begin{CJK}{UTF8}{gbsn}
        他们 前来 学画 ， 除了 出于 对 \colorbox[rgb]{0.97, 0.82, 0.80}{中国} 文化 的 仰慕 之外 ， 另 一 重要 原因 就 是 排解 心中 的 寂寞 。
        \end{CJK}
        \\
        \multirow{2}{*}{Chinese} & \textbf{Ours: }
        \begin{CJK}{UTF8}{gbsn}
        他们 前来 学画 ， 除了 出于 对 \colorbox[rgb]{0.80, 0.98, 0.85}{[{\scriptsize LOC} 中国]} 文化 的 仰慕 之外 ， 另 一 重要 原因 就 是 排解 心中 的 寂寞 。
        \end{CJK}
        \\
        & \textbf{Translation in English: }\colorbox[rgb]{1, 1, 1}{In addition to the admiration for the culture of China, they came here to learn painting for another important}\\
        & reason, that is, dispelling the loneliness in their hearts.\\
    \hline
    
    \end{tabular}
    \end{adjustbox}
    \caption{Results of unsupervised cross-lingual NER. The \colorbox[rgb]{0.80, 0.98, 0.85}{GREEN} (\colorbox[rgb]{0.97, 0.82, 0.80}{RED}) highlight indicates a correct (incorrect) label.}
    \label{tab:sup_case_study}
\end{table*}

\begin{table*}[hb]
  \centering
    \setlength{\tabcolsep}{1mm}
    \begin{adjustbox}{max width=\textwidth}
    \begin{tabular}{l|c|c|c|c|c|c}
      \hline
         &  es  &   nl  &   de  &   fr  &   zh  & Average\\ \hline
        % \textbf{Ours} &   \textbf{80.32}  &   \textbf{83.72}  &   \textbf{77.70}  &   \textbf{69.19}  &   85.67   &   \textbf{79.32} \\ \hline
        Ours &  80.32   &   83.72   &   77.70   &   69.19   &   85.67   &   79.32 \\ \hline
        Ours w/o max loss &79.76 (-0.56) &  82.89 (-0.83) & 76.54 (-1.16) & 67.55 (-1.64) & 86.00 (0.33) &  43.17 (-0.77    )\\ \hline
        Ours w/o masking    &   79.54 (-0.78) & 83.47 (-0.25) & 77.28 (-0.42) & 68.96 (-0.23) & 85.44 (-0.23) & 43.67 (-0.38    )\\ \hline
        Ours w/o max loss/masking & 78.99 (-1.33) & 82.94 (-0.78) & 76.63 (-1.07) & 67.88 (-1.31) & 85.59 (-0.08) & 43.06 (-0.91    )\\ \hline
        Ours w/o meta-train/max loss/masking    &\multirow{2}{*}{78.74 (-1.58)} &   \multirow{2}{*}{82.00 (-1.72)} &    \multirow{2}{*}{75.48 (-2.22)} &    \multirow{2}{*}{67.73 (-1.46)} &    \multirow{2}{*}{85.11 (-0.56)} &    \multirow{2}{*}{42.45 (-1.51)} \\
        % Ours w/o meta-train/max loss/masking  &78.74 (-1.58) &    82.00 (-1.72) & 75.48 (-2.22) & 67.73 (-1.46) & 85.11 (-0.56) & 42.45 (-1.51    ) \\ \hline
        \multicolumn{1}{c|}{(\ie, Base Model)} & & & & & \\
        \hline
    \end{tabular}
    \end{adjustbox}
    \caption{Ablation study on low-resource cross-lingual NER with 5\% training data in target languages.}%``$-$" denotes removing the corresponding strategies.}
    \label{tab:sup_ablation}
\end{table*}
